# Supplementary material for: Are Web Agents Still Detectable? Stress-Testing Bot Defenses with Coordinated Evasion
Source: arXiv:2611.31962 source file (2026-12-01)
Supplement: Supplementary file 1 [file appendix.tex]

\section{Appendix}
\label{sec:appendix}

\noindent\textbf{Latent space analysis.}
We examine whether nearby latent vectors produce consistent typing behavior using a TypeNet-style embedding model. On split 2, we sample 128 base latents and generate samples with progressively larger latent perturbations. We measure cosine similarity between their typing embeddings for both repeated generations of the same target and generations of different targets. Figure~\ref{figure:latent-style} shows that similarity decreases as perturbation increases in both settings, suggesting that nearby latents preserve aspects of typing behavior. This also suggests the potential for controllable generation by steering the latent toward specific behaviors, such as typing speed or error frequency.

\noindent\textbf{Baseline availability.}
We considered BeCAPTCHA-Mouse~\cite{acien2022becaptcha} and
DMTG~\cite{liu2024dmtg} as additional generative baselines. We contacted
the BeCAPTCHA-Mouse authors to request their trajectory-generation code
and benchmark data on October~2 and sent a follow-up on October~9,
but had received no response as of November~2.
For DMTG, we could not locate a public implementation or reproduce the
generator from the available documentation. We therefore
do not report direct experimental comparisons with these generators.
