# Supplementary material for: Are Web Agents Still Detectable? Stress-Testing Bot Defenses with Coordinated Evasion
Source: arXiv:2611.31962 source file (2026-12-01)
Supplement: Supplementary file 2 [file ethical-considerations.tex]

% \section{Ethical Considerations}
% \label{app:ethics}

% \noindent\textbf{Dual-use risks and benefit--harm assessment.}
% Our stakeholders include website operators, legitimate users whose access
% anti-bot gates mediate, security vendors whose protections we evaluate,
% participants in the public interaction corpora we analyze, and defensive
% researchers. Studying coordinated evasion carries clear dual-use risk: a
% browser that suppresses automation artifacts paired with human-trained motor
% generators could lower the cost of unauthorized scraping, credential stuffing,
% bulk account creation, or automated fraud. Secondary risks include unintended
% traffic load on live websites during measurement and biometric re-identification
% in human interaction logs.

% We weighed these risks against the defensive harm of evaluating bot detectors
% only against uncoordinated baselines. Released detectors (\FPAgent and
% AgentShield) report near-perfect accuracy on default agents, yet our
% measurements show that coarse interaction counts and host-specific fingerprints
% fail against heuristic or generative mimicry and unseen execution hosts.
% Documenting these failure modes at the architectural level helps defenders
% audit and harden multi-channel detection. Releasing \MimicTrace alongside
% concrete cross-channel, runtime, and boundary-timing checks while withholding
% turnkey offensive tooling keeps a deployable evasion stack out of public
% circulation.

% \noindent\textbf{Controlled testbed isolation.}
% All component comparisons ($540$ sessions in Table~\ref{tab:matrix}),
% server-verified form evaluations ($40$ live trials in Tables~\ref{tab:agentshield}
% and~\ref{tab:mimictrace-summary}), and multi-channel audits ($172$ honeysite
% sessions and $14$ stock-browser controls in Table~\ref{tab:mimictrace-channels})
% ran exclusively on synthetic web services hosted on our own local infrastructure.
% These experiments created no third-party accounts, conducted no transactions,
% collected no external user data, and kept CAPTCHA solving disabled on the
% honeysite.

% \noindent\textbf{Live-site evaluation.}
% Before testing any live website, we sought sanctioned vendor evaluation
% environments. In August~2026, we contacted DataDome, Kasada, Akamai, and Shape
% to request research testbeds or authorized evaluation access and received no
% response. Without a sanctioned testbed, we ran the public 80-task Stealth
% Bench~V1 suite~\cite{stealthbenchv1} once on August~21, 2026, as it already
% benchmarks commercial browser providers on public pages and provides the only
% reproducible external reference for deployed defenses. Every task was capped at
% a single run and limited to unauthenticated browsing open to any visitor (site
% search, opening a public page, and reading a link). When a site presented a
% CAPTCHA or interactive challenge during that attempt, the agent interacted with
% it within the single task run. The agent logged into no accounts, submitted no
% forms beyond public search queries, made no purchases, posted no content, and
% retained no scraped site content; our analysis records only the binary block
% outcome per task.

% \noindent\textbf{Vendor disclosure.}
% Following our evaluation, we notified the contacted anti-bot vendors with an
% aggregate summary of our Stealth Bench~V1 access outcomes and technical
% descriptions of the evasion mechanisms relevant to their products (out-of-renderer
% control, world-gated observation, native input delivery, cross-channel persona
% alignment, and generative mouse/keyboard synthesis), together with the
% runtime and boundary signals that remained informative in our audit, without
% distributing turnkey patches or exploit code. We remain available to coordinate
% technical follow-up with any vendor that responds prior to publication.

% \noindent\textbf{Human data.}
% We collected no new human-subjects data in this study. Our behavioral models
% train and evaluate exclusively on publicly released corpora used under their
% published terms: the Bo\u{g}azi\c{c}i Mouse Dynamics
% Dataset~\cite{kilic2021bogazici}, the Aalto free-text keystroke
% corpus~\cite{dhakal2018typing}, and the Attentive Cursor
% Dataset~\cite{leiva2020attentive}. \MimicTrace's human reference records come
% from the publicly released logs of \FPAgent~\cite{wang2026fpagent} and
% AgentShield~\cite{agentshield}, from which we derive features solely over their
% recorded fields without pooling unrelated corpora or attempting participant
% re-identification. Only aggregate statistics and anonymized session summaries
% are reported.

% \noindent\textbf{Release policy.}
% While Section~\ref{sec:darkagent} describes the full \DarkAgent, \Browsium, and
% \Behavium architectures so defenders can evaluate and build countermeasures
% against them, we restrict artifact release to prevent turnkey misuse: we
% publicly release \MimicTrace and all defensive measurement and evaluation code,
% while withholding deployable attack code, source-level \Browsium stealth
% patches, trained \Behavium generator weights, and operational attack
% configurations (Appendix~\ref{app:open-science}).



\section{Ethical Considerations}
\label{app:ethics}

\noindent\textbf{Risks and benefits.}
\DarkAgent could facilitate unauthorized scraping, credential stuffing,
bulk account creation, and fraud, harming website operators and users
through privacy violations, financial loss, and increased service costs.
Our results make misuse credible but do not estimate its likelihood or
scale. They also expose limitations in detecting coordinated browser and
behavioral adaptation, motivating stronger defensive evaluation.
We will release \MimicTrace while withholding operational \DarkAgent
artifacts. This reduces direct enablement but cannot prevent reconstruction
from the paper or adversarial tuning against the benchmark. We judge the
benefits of independent defensive evaluation to outweigh these residual risks.

\noindent\textbf{Controlled experiments.}
Component comparisons, form-completion trials, and multi-channel audits
(Tables~\ref{tab:matrix}, \ref{tab:agentshield},
\ref{tab:mimictrace-summary}, and~\ref{tab:mimictrace-channels})
ran on synthetic services hosted on our own infrastructure. They created no
third-party accounts, conducted no transactions, and collected no external
user data. CAPTCHA solving remained disabled on the honeysite.

\noindent\textbf{Live-site evaluation.}
In August~2026, we requested research testbeds or authorized access from
DataDome, Kasada, Akamai, and Shape, receiving no response. These requests
did not establish authorization. To measure deployed access decisions
unavailable in our controlled experiments, we ran the 80-task Stealth Bench~V1
suite~\cite{stealthbenchv1} once on August~21, 2026, with one run per task.
Tasks involved unauthenticated browsing and public searches, including
interaction with challenges encountered during the run. The agent logged
into no accounts, submitted no forms beyond search queries, made no
purchases, and posted no content. We retained binary block outcomes, not
scraped site content. These restrictions reduced potential harm but did not
eliminate the ethical risks of testing without explicit operator consent.


\noindent\textbf{Human data and privacy.}
We use public Bo\u{g}azi\c{c}i~\cite{kilic2021bogazici},
Aalto~\cite{dhakal2018typing}, and Attentive
Cursor~\cite{leiva2020attentive} datasets under their published terms,
with human reference logs from \FPAgent~\cite{wang2026fpagent} and
AgentShield~\cite{agentshield}. We neither link participants across datasets
nor attempt re-identification. Because behavioral traces may remain
identifying after direct identifiers are removed, released data will undergo
privacy and redistribution review. We will document exclusions and provide
acquisition instructions for restricted third-party data where permitted.


\noindent\textbf{Defensive mitigation.}
\MimicTrace's cross-channel, runtime, and boundary-timing checks support
complementary detection. Defenders should validate them on unseen clients
and tasks, combine them with rate limits and account-level controls, and
assess false positives, privacy, and accessibility. 
