# Supplementary material for: Are Web Agents Still Detectable? Stress-Testing Bot Defenses with Coordinated Evasion
Source: arXiv:2611.31962 source file (2026-12-01)
Supplement: Supplementary file 3 [file open-science.tex]

% \section{Open Science}

% During review, the submission artifact will provide an anonymized repository;
% after de-anonymization, the same materials will be released through a public
% GitHub repository and companion GitHub Pages application. The repository will
% contain the controlled websites, execution validators, task definitions,
% evaluation orchestration, prompts and model budgets, environment manifests,
% preprocessing code, and statistical-analysis scripts for all reproducible
% non-commercial experiments. It will pin source commits, dependency versions,
% detector configurations, random seeds, feature definitions,
% dataset-specific split manifests, model hyperparameters, and checkpoints.
% The split manifests identify the grouping actually used: verified
% participant identities where available, and persistent browser
% identifiers for the \FPAgent data when participant mappings are
% unavailable.
% Per-trial CSV/JSON outcomes will accompany every reported controlled result with a manifest linking each table cell to its source
% artifact. The web application will expose aggregate tables, experiment
% metadata, and links to the corresponding code and results.

% Detector artifacts will be redistributed only when their licenses permit;
% otherwise the repository will provide retrieval and configuration instructions.
% Commercial systems and human traces that cannot be released will be documented
% with sufficient metadata, aggregate outcomes, and justified restrictions. Any
% withheld \DarkAgent component will be listed explicitly with the ethical,
% licensing, or misuse rationale for the omission.

\section{Open Science}
\label{app:open-science}

For artifact inquiries, contact Parsa Nilforushan
at \href{mailto:parsa_nilforushan@sfu.ca}{\nolinkurl{parsa_nilforushan@sfu.ca}}.
